# Supplementary material for: Evolution and learning in differentiable robots
Source: arXiv:2405.14712 source file (2024-05-26)
Supplement: Supplementary file 1 [file 7_Appendix.tex]

\section{Appendix}
\label{sec:appendix}

This appendix contains 
one table (Table~\ref{table:resin})
% three tables (Tables~\ref{table:resin}, \ref{table:robot-size} and \ref{table:robot-active-frac})
and one plot (Fig.~\ref{fig:population-fitness}). 
Fig.~\ref{fig:population-fitness} is similar to Fig.~\ref{fig:fitness} but tracks the mean fitness ($\pm$1 S.D.) of the population instead of the fitness of the best design in the population, at every generation.
% Table~\ref{table:robot-size} displays the size of the robots in terms of spring count, 
% and Table~\ref{table:robot-active-frac} shows the fraction of those springs that are motorized, at the beginning and end of evolution.
Table~\ref{table:resin} displays the material properties of the particular resin we used to 3D print the robots.
